# Supplementary material for: Cooperating RPN's Improve Few-Shot Object Detection
Source: arXiv:2011.10142 source file (2020-11-19)
Supplement: Supplementary file 1 [file supp.tex]

\section{Implementation Details}
\label{impl_details}
Following \citet{wang2020few}, we use Faster R-CNN as our base model and use an ImageNet pre-trained \citep{russakovsky2015imagenet} ResNet-101 with a Feature Pyramid Network \citep{lin2017feature} as the backbone. Our model takes roughly the same training time as \citet{wang2020few}. All training and fine-tuning hyperparameters (batch size, learning rate, momentum, weight decay, etc.) are the same as \citet{wang2020few}. CoRPNs have the following additional hyperparameters: the number of RPN's, the cooperation loss threshold $\phi$, the diversity loss trade-off $\lambda_{d}$, and the cooperation loss trade-off $\lambda_{c}$. We mostly use five RPN's, except for PASCAL VOC novel split 3, where two RPN's lead to better performance. We showed the effect of using different levels of $\phi$ in ablation studies of the main paper. In general, $\phi$ $\in$ $[0.1, 0.3]$ works best. In addition, results are relatively stable for $\lambda_{c}$ $\in$ $[0.5, 2]$ and $\lambda_{d}$ $\in$ $[0.01, 0.1]$. The number of RPN's also affects the stable interval, for PASCAL VOC split 3, with 2 RPN's, we find that $\lambda_{d}$ $\in$ $[0.1, 0.2]$ works the best.

As discussed in the main paper, the training process of CoRPNs is two-phase. Our training and fine-tuning procedures are consistent with \citet{wang2020few}. On PASCAL VOC, at phase 1 base classes training, each model is trained on the union set of VOC 07+12 trainval data. Evaluation is on the VOC 07 test set. At the fine-tuning phase, each model is fine-tuned with a balanced few-shot dataset sampled from VOC 07+12 that contains both base classes and novel classes. On COCO, the fine-tuning phase is two-stage: at stage 1, we fine-tune the model on novel classes; at stage 2, we then fine-tune the model with a balanced few-shot dataset containing both base and novel classes. 

As mentioned in the main paper, we use the standard evaluation procedure for all the compared models for a fair comparison. We also compare against other approaches with the same novel classes instances and test images. On COCO, We fine-tuned and re-evaluated the publicly released models of MPSR \citep{wu2020mpsr} and FSDetView \citep{Xiao2020FSDetView} with the same novel classes instances in \citet{wang2020few}. In the standard evaluation procedure, when a test image comes in, the model has no assumption on what categories the image contains. We re-evaluated FSOD \citep{fan2020fsod} and CoAE \citep{Hsieh19AttenFew} using the standard evaluation. In \citet{wang2020few} and CoRPNs, the classifier is a $(|C_b| + |C_n|)$-way classifier. FSOD replaces it with a class-agnostic 2-way classifier, which only determines if an object is foreground or background. At inference time, FSOD produces a balanced number of proposals per novel category and concatenates these proposals before NMS. In the standard evaluation, we produce a balanced number of proposals for every category, including base categories. In CoAE, for a test image containing a certain category, CoAE samples support image(s) from this category and collects boxes based on the support image(s). We modify the inference process by providing each test image support image(s) from each category and performing a forward pass for all categories. We then collect boxes from all categories and evaluate them. For a fair comparison, for the results reported in the main paper, we also fine-tuned FSOD and CoAE with the same novel category instance(s) as in \citet{wang2020few} and CoRPNs.%published rpre-trained weights
 
% \paragraph{Evaluating Few-Shot Detectors} \wl{todo}
% table 1 and 2 
%This table shows the *Model extended from tracking-like setting to open-world setting. Notice that ours substantially outperforms baseline \citep{wang2020few} in very few-shot settings and retains comparable performance on higher-shots. Ours outperforms other SOTA detectors on shots 1 and 2, and retains comparable performance on higher-shots for a fair comparison

% how we only pick one class-aware framework to compare with (among repmet, CoAE, os2d)

\section{Results on Base classes}
CoRPNs use a two-phase approach like TFA \citep{wang2020few}. Here we provide the base classes AP after phase 1 base classes training. As shown in Tables~\ref{tab:voc_stage1} and~\ref{tab:coco_stage1}, our performance on base classes is comparable with TFA \citep{wang2020few}. Note that the setting of Tables~\ref{tab:voc_stage1} and~\ref{tab:coco_stage1} is different from that of Table 3 (COCO base classes) in the main paper, where the results are reported after phase 2 $k$-shot novel classes fine-tuning.

\begin{minipage}[b]{0.49\textwidth}
  \centering

\resizebox{\linewidth}{!}{\begin{tabular}{lccc}
    \toprule
    % \multicolumn{2}{c}{Part}                   \\
    % \cmidrule(r){1-2}
    Method & Split 1 & Split 2& Split 3\\
    \midrule
    TFA w/ cos ~\citep{wang2020few} &  80.8 & \bf81.9 & 82.0	   \\
    CoRPNs w/ cos (Ours) & 	\bf81.2&  81.8 & \bf82.4 \\
    \bottomrule
    \vspace{-3mm}
  \end{tabular}}%
 \captionof{table}{Base classes AP50 on PASCAL VOC after phase 1 base class training. The same parameter setting applies to both models. Notice that ours is comparable to the results of TFA.}%This table presents the 
 \label{tab:voc_stage1}
 \end{minipage}
 \quad
 \begin{minipage}[b]{0.47\textwidth}
 \centering

\resizebox{\linewidth}{!}{\begin{tabular}{lccc}
    \toprule
    % \multicolumn{2}{c}{Part}                   \\
    % \cmidrule(r){1-2}
    Method & AP & AP50 & AP75\\
    \midrule
    TFA w/ cos ~\citep{wang2020few} &  \bf39.2 & 59.3 & \bf42.8	   \\
    CoRPNs w/ cos (Ours) & 	\bf39.2&  \bf59.4 & 42.5 \\
    \bottomrule
    \vspace{-3mm}
    \label{tab:coco_stage1}
  \end{tabular}}
\captionof{table}{Base classes AP, AP50, and AP75 on COCO after phase 1 base class training. The same parameter setting applies to both models. Ours is comparable to the reported numbers of TFA.}
\label{tab:coco_stage1}
\end{minipage}

\section{Error Analysis}
We provide some proposal and final detection visualizations of CoRPNs and TFA \citep{wang2020few} on PASCAL VOC. Specifically, Figure~\ref{vis_proposal_detection} presents the proposals and the detection results for cat test images from 1-shot fine-tuned models under base/novel split 3. Cat is a novel category for this split. TFA fails to generate proper proposals, so that all cat boxes are missed in the final detection. CoRPNs fix the proposal neglect effect and detect many more cat objects. However, since the few-shot classifier is weak on novel classes, and the classifier has engaged with strong priors with base classes, cats are often misclassified as other base categories, leading to a performance drop. This suggests that if we have a better classifier, we can further improve the performance. 
\begin{figure}[h]
\centering
\includegraphics[width=\linewidth]{} \\
\includegraphics[width=\linewidth]{} \\
\vspace{0.2cm}
\includegraphics[width=\linewidth]{} \\
\includegraphics[width=\linewidth]{} \\
\vspace{1mm}
\caption{Top 10 proposals and final detection results of TFA \citep{wang2020few} (proposal {\bf row 1}; detection {\bf row 3}) and CoRPNs (proposal {\bf row 2}; detection {\bf row 4}). Note that the proposals produced by TFA are tiny boxes. All images here are {\bf cat} (cat is a novel category) test images. Due to the proposal neglect effect, state-of-the-art TFA misses all cat boxes. By contrast, CoRPNs catch many more cat objects by eliminating the effect, thus significantly outperforming TFA. However, we also notice that CoRPNs still have difficulty of correctly classifying the proposals as cats, suggesting that improving the classifier will further boost the detection performance, which we leave as future work.}
\label{vis_proposal_detection}
\end{figure}

\begin{figure}[hbt!]
\centering
\includegraphics[width=\linewidth]{} \\
\includegraphics[width=\linewidth]{} \\
\vspace{0.15cm}
\includegraphics[width=\linewidth]{} \\
\includegraphics[width=\linewidth]{} 
\vspace{-3mm}
\caption{Detection results of TFA \citep{wang2020few} ({\bf row 1 \& 3}) and CoRPNs ({\bf row 2 \& 4}) under PASCAL VOC split 1 shot 1 ({\bf row 1 \& 2}), and split 3 shot 1 ({\bf row 3 \& 4}). Novel classes shown here are \{bird, bus, cow, boat, cat, motorbike, sheep, sofa\}. TFA fails to detect many novel objects due to the proposal neglect effect, while our CoRPNs catch many more novel objects by eliminating the effect.}
\label{vis}
\end{figure}

\begin{figure}[h]
\centering
\includegraphics[width=\linewidth]{} \\
\includegraphics[width=\linewidth]{} \\
\vspace{0.2cm}
\includegraphics[width=\linewidth]{} \\
\includegraphics[width=\linewidth]{} \\
\vspace{0.2cm}
\includegraphics[width=\linewidth]{} \\
\includegraphics[width=\linewidth]{} \\
\vspace{1mm}
\caption{Detection results of TFA \citep{wang2020few} ({\bf row 1 \& 3 \& 5}) and CoRPNs ({\bf row 2 \& 4 \& 6}) under COCO test sets (val2014). Novel classes shown here are \{airplane, bird, boat, bottle, bus, cat, cow, horse, motorcycle, person, train\}. TFA fails to detect many novel objects due to the proposal neglect effect, while our CoRPNs catch many more novel objects by eliminating the effect.}
\label{vis_coco}
\end{figure}

\section{PASCAL VOC Visualizations}
We provide novel object detection result visualizations of CoRPNs and TFA \citep{wang2020few} on PASCAL VOC in Figure~\ref{vis}. TFA reflects the proposal neglect effect and misses lots of novel objects, while CoRPNs detect many more novel objects.  
\section{COCO Visualizations}
We provide additional novel object detection result visualizations of CoRPNs and TFA \citep{wang2020few} on COCO in Figure~\ref{vis_coco}. Again, TFA fails to detect many novel objects due to the proposal neglect effect, whereas CoRPNs catches many more novel objects by eliminating the effect.
